# Supplementary material for: Extracting maximum power from active colloidal heat engines
Source: arXiv:1803.01620 ancillary file (2018-04-23)
Supplement: Supplementary file 1 [file SI.pdf]

# Supplementary material: Extracting maximum power from active colloidal heat engines

D. Martin[1,2], C. Nardini[1,3], M. E. Cates[1] and É. Fodor[1]

[1] *DAMTP, Centre for Mathematical Sciences, University of Cambridge, Wilberforce Road, Cambridge CB3 0WA, UK*
[2] *Université Paris Diderot, Sorbonne Paris Cité, MSC, UMR 7057 CNRS, 75205 Paris, France*
[3] *Service de Physique de l'État Condensé, CNRS UMR 3680, CEA-Saclay, 91191 Gif-sur-Yvette, France*

PACS `05.70.Ln` – Nonequilibrium and irreversible thermodynamics
PACS `05.40.-a` – Fluctuation phenomena, random processes, noise and Brownian motion
PACS `82.70.Dd` – Colloids

**Abstract** – Supplementary data to "Extracting maximum power from active colloidal heat engines".

**Coarse-grained bath dynamics.** – From the microscopic dynamics in (1) of the main text, the coarse-grained dynamics of the bath density $\rho(\mathbf{r},t)=\sum_i \delta[\mathbf{r}-\mathbf{r}_i(t)]$ reads [1]

$$\begin{aligned}\partial_t\rho(\mathbf{r},t) = \mu\nabla_{\mathbf{r}}\cdot\left[\rho(\mathbf{r},t)\int\rho(\mathbf{r}',t)\nabla_{\mathbf{r}}V(\mathbf{r}-\mathbf{r}')\mathrm{d}\mathbf{r}'+\rho(\mathbf{r},t)\nabla_{\mathbf{r}}U(\mathbf{r}-\mathbf{x})+T\nabla_{\mathbf{r}}\rho(\mathbf{r},t)\right]\\ +\nabla_{\mathbf{r}}\cdot\left[\sqrt{2\mu\rho(\mathbf{r},t)T}\boldsymbol{\Lambda}(\mathbf{r},t)\right].\end{aligned} \tag{S1}$$

The fluctuating term $\boldsymbol{\Lambda}$ is a zero-mean Gaussian noise with correlations $\langle\Lambda_\alpha(\mathbf{r},t)\Lambda_\beta(\mathbf{r}',t')\rangle=\delta_{\alpha\beta}\delta(\mathbf{r}-\mathbf{r}')\delta(t-t')$. We consider density fluctuations $\delta\rho=\rho-\rho_0$ around the average density $\rho_0$. By assuming that both the bath-bath and the bath-tracer interactions are weak, we deduce the dynamics of the density mode $\delta\rho_{\mathbf{k}}(t)=\int\delta\rho(\mathbf{r},t)\mathrm{e}^{\mathrm{i}\mathbf{k}\cdot\mathbf{r}}\mathrm{d}\mathbf{r}$ as

$$\partial_t\delta\rho_{\mathbf{k}} = -\mu\mathbf{k}^2(T+\rho_0V_{\mathbf{k}})\delta\rho_{\mathbf{k}}-\mu\mathbf{k}^2\rho_0U_{\mathbf{k}}\mathrm{e}^{\mathrm{i}\mathbf{k}\cdot\mathbf{x}}+\sqrt{2\mu\rho_0T}\mathrm{i}\mathbf{k}\cdot\boldsymbol{\Lambda}_{\mathbf{k}}, \tag{S2}$$

yielding

$$\delta\rho_{\mathbf{k}}(t)=\int\mathrm{d}s\mathcal{G}_{\mathbf{k}}(t-s)\left[\sqrt{2\mu\rho_0T}\mathrm{i}\mathbf{k}\cdot\boldsymbol{\Lambda}_{\mathbf{k}}(s)-\mu\mathbf{k}^2\rho_0U_{\mathbf{k}}\mathrm{e}^{\mathrm{i}\mathbf{k}\cdot\mathbf{x}(s)}\right], \tag{S3}$$

where $\mathcal{G}_{\mathbf{k}}(t)=\mathrm{e}^{-\mu\mathbf{k}^2(T+\rho_0V_{\mathbf{k}})t}\Theta(t)$, and $\Theta$ refers to the Heaviside step function. The linearization of the bath dynamics can be regarded as a mean-field treatment of interactions valid for both weak interactions and high density [2].

**Effective tracer dynamics.** – We follow the procedure detailed in [2,3] to derive the effective tracer dynamics. The force exerted by the bath on the tracer reads

$$-\nabla_{\mathbf{x}}\sum_i U(\mathbf{r}_i-\mathbf{x})=\int \mathrm{i}\mathbf{k}U_{\mathbf{k}}\mathrm{e}^{-\mathrm{i}\mathbf{k}\cdot\mathbf{x}}\frac{\mathrm{d}\mathbf{k}}{(2\pi)^d}, \tag{S4}$$

where $d$ refers to the spatial dimension. It can be written as

$$-\nabla_{\mathbf{x}}\sum_i U(\mathbf{r}_i-\mathbf{x})=\boldsymbol{\xi}-\int\frac{\mathrm{d}\mathbf{k}}{(2\pi)^d}\mathrm{i}\mathbf{k}U_{\mathbf{k}}\mathrm{e}^{-\mathrm{i}\mathbf{k}\cdot\mathbf{x}(t)}\int \mathrm{d}s\mathcal{G}_{\mathbf{k}}(t-s)\mu\mathbf{k}^2\rho_0U_{\mathbf{k}}\mathrm{e}^{\mathrm{i}\mathbf{k}\cdot\mathbf{x}(s)}, \tag{S5}$$

where

$$\boldsymbol{\xi}[\mathbf{x}(t),t]=\int\frac{\mathrm{d}\mathbf{k}}{(2\pi)^d}\mathrm{i}\mathbf{k}U_{\mathbf{k}}\mathrm{e}^{-\mathrm{i}\mathbf{k}\cdot\mathbf{x}(t)}\int \mathrm{d}s\mathcal{G}_{\mathbf{k}}(t-s)\sqrt{2\mu\rho_0T}\mathrm{i}\mathbf{k}\cdot\boldsymbol{\Lambda}_{\mathbf{k}}(s). \tag{S6}$$

The term $\boldsymbol{\xi}$ reflects the effect of the bath noise into the tracer dynamics, the next term in (S5) embodies the effect of the tracer in the surrounding bath, which in turn resists the tracer motion. Such noise and damping terms contain some memory effects which depend on the tracer position. We evaluate the noise correlations as

$$\begin{aligned}\langle\xi_\alpha[\mathbf{x}(t),t]\xi_\beta[\mathbf{x}(t'),t']\rangle=2\mu\rho_0T&\int\frac{\mathrm{d}\mathbf{k}}{(2\pi)^d}k_\alpha k_a U_{\mathbf{k}}\mathrm{e}^{-\mathrm{i}\mathbf{k}\cdot\mathbf{x}(t)}\int\mathrm{d}s\mathcal{G}_{\mathbf{k}}(t-s)\\&\times\int\frac{\mathrm{d}\mathbf{q}}{(2\pi)^d}q_\beta q_b U_{\mathbf{q}}\mathrm{e}^{-\mathrm{i}\mathbf{q}\cdot\mathbf{x}(t')}\int\mathrm{d}s'\mathcal{G}_{\mathbf{q}}(t'-s')\langle\Lambda_{a,\mathbf{k}}(s)\Lambda_{b,\mathbf{q}}(s')\rangle,\end{aligned} \tag{S7}$$

yielding

$$\begin{aligned}\langle\xi_\alpha[\mathbf{x}(t),t]\xi_\beta[\mathbf{x}(t'),t']\rangle&=\delta_{\alpha\beta}\frac{2\mu\rho_0T}{d}\int\frac{\mathrm{d}\mathbf{k}}{(2\pi)^d}\mathbf{k}^4U_{\mathbf{k}}^2\mathrm{e}^{-\mathrm{i}\mathbf{k}\cdot[\mathbf{x}(t)-\mathbf{x}(t')]}\int\mathrm{d}s\mathcal{G}_{\mathbf{k}}(t-s)\mathcal{G}_{\mathbf{k}}(t'-s)\\&=\delta_{\alpha\beta}\frac{\rho_0T}{d}\int\frac{\mathrm{d}\mathbf{k}}{(2\pi)^d}\frac{\mathbf{k}^2U_{\mathbf{k}}^2}{T+\rho_0V_{\mathbf{k}}}\mathrm{e}^{-\mathrm{i}\mathbf{k}\cdot[\mathbf{x}(t)-\mathbf{x}(t')]-\mu\mathbf{k}^2(T+\rho_0V_{\mathbf{k}})|t-t'|},\end{aligned} \tag{S8}$$

where we have used that both $U_{\mathbf{k}}$ and $\mathcal{G}_{\mathbf{k}}$ are symmetric with respect to $\mathbf{k}$. To proceed further, we assume that the variations of tracer position are slow compared with the typical relaxation time of the bath. The tracer position relaxes in the harmonic trap in a time $\kappa^{-1}$ when it is isolated from surrounding particles. The bath relaxation operates through diffusion in a time $\tau_{\mathrm{diff}}=\sigma^2/\mu(T+\rho_0V_{|\mathbf{k}|=0})$ on the tracer scale $\sigma$. Then, the adiabatic approximation $\kappa\tau_{\mathrm{diff}}\ll 1$ allows one to neglect the dependence of the noise correlations on the tracer position:

$$\begin{aligned}\langle\xi_\alpha[\mathbf{x}(t),t]\xi_\beta[\mathbf{x}(t'),t']\rangle&\simeq\langle\xi_\alpha[\mathbf{x}(t),t]\xi_\beta[\mathbf{x}(t),t']\rangle\\&\simeq\delta_{\alpha\beta}\frac{\rho_0T}{d}\int\frac{\mathrm{d}\mathbf{k}}{(2\pi)^d}\frac{\mathbf{k}^2U_{\mathbf{k}}^2}{T+\rho_0V_{\mathbf{k}}}\mathrm{e}^{-\mu\mathbf{k}^2(T+\rho_0V_{\mathbf{k}})|t-t'|}.\end{aligned} \tag{S9}$$

Accounting for the bath-tracer interactions via a Gaussian potential of the form $U(\mathbf{x})=U_0\mathrm{e}^{-(\mathbf{x}/\sigma)^2/2}$, and neglecting the spatial extension of bath particles: $V_{\mathbf{k}}\simeq V_{|\mathbf{k}|=0}$, we can evaluate the noise correlations as

$$\langle\xi_\alpha(t)\xi_\beta(0)\rangle=\delta_{\alpha\beta}\frac{\Omega_d\Gamma(1+d/2)}{2d}\frac{\rho_0\sigma^{2d}U_0^2T/(T+\rho_0V_{|\mathbf{k}|=0})}{[\sigma^2+\mu(T+\rho_0V_{|\mathbf{k}|=0})|t|]^{1+d/2}}, \tag{S10}$$

where $\Gamma$ is the Gamma function, and $\Omega_d=2\pi^{d/2}/\Gamma(d/2)$ refers to the solid angle in $d$ dimension. Alternatively, the noise correlations can be written as

$$\langle\xi_\alpha(t)\xi_\beta(0)\rangle=\delta_{\alpha\beta}\frac{\pi^{d/2}\rho_0\sigma^dU_0^2T/\sigma^2/(T+\rho_0V_{|\mathbf{k}|=0})}{2(1+|t|/\tau_{\mathrm{diff}})^{1+d/2}}. \tag{S11}$$

The correlations of the force exerted by the bath on the tracer have some power-law decay with exponent $1{+}d/2$ depending on spatial dimension $d$. Within the adiabatic approximation $\kappa\tau_{\rm diff} \ll 1$, we further neglect the time dependence of the noise correlations:

$$\langle \xi_\alpha(t)\xi_\beta(0)\rangle \simeq \delta_{\alpha\beta}\delta(t)\frac{\pi^{d/2}\rho_0\sigma^d U_0^2 T}{2\sigma^2(T+\rho_0 V_{|\mathbf{k}|=0})}\int_{-\infty}^{\infty}\frac{{\rm d}t'}{(1+|t'|/\tau_{\rm diff})^{1+d/2}}, \tag{S12}$$

yielding $\langle \xi_\alpha(t)\xi_\beta(0)\rangle = 2\lambda T\delta_{\alpha\beta}\delta(t)$, where

$$\lambda = \frac{\pi^{d/2}\rho_0\sigma^d U_0^2}{\mu d(T+\rho_0 V_{|\mathbf{k}|=0})^2}. \tag{S13}$$

For arbitrary potentials, one can also derive a generic expression for $\lambda$ in the adiabatic limit $\kappa\tau_{\rm diff} \ll 1$ directly from (S9) as

$$\lambda = \frac{\rho_0}{\mu d}\int \frac{{\rm d}\mathbf{k}}{(2\pi)^d}\left[\frac{U_\mathbf{k}}{T+\rho_0 V_\mathbf{k}}\right]^2. \tag{S14}$$

Given that the bath formed by the passive Brownian particles is an equilibrium bath, the corresponding noise and damping terms in the tracer dynamics should fulfill the fluctuation-dissipation theorem [4]. The effective tracer dynamics follows as given by (5) of the main text.

**Average extracted work and output power.** – Engines A and B described in the main text operate with the following four successive branches

- the trap stiffness increases linearly in time during the compression interval $[0,\Delta t/2]$ at low temperature (small persistence): $\kappa(t) = 2(\kappa_{\rm M}-\kappa_{\rm m})t/\Delta t + \kappa_{\rm m}$,
- the temperature (persistence) increases instantaneously at fixed trap stiffness,
- the trap stiffness decreases linearly in time during the expansion interval $[\Delta t/2,\Delta t]$ at high temperature (large persistence): $\kappa(t) = 2(\kappa_{\rm m}-\kappa_{\rm M})t/\Delta t + \kappa_{\rm M}$,
- the temperature (persistence) decreases instantaneously at fixed trap stiffness.

The average extracted work reads $\mathcal{W} = (1/2)\int_0^{\Delta t}\dot\kappa\langle\mathbf{x}^2\rangle{\rm d}t$. Noting that the self-propulsion dynamics can be written as $\tau\dot{\mathbf{f}} = -\mathbf{f}+\boldsymbol{\zeta}$, where $\boldsymbol{\zeta}$ is a zero-mean Gaussian white noise uncorrelated with $\{\boldsymbol{\eta}\}_i$ and with correlations $\langle\zeta_\alpha(t)\zeta_\beta(0)\rangle = 2T\delta_{\alpha\beta}\delta(t)$, we use Itô calculus to get

$$\begin{aligned}
\frac{{\rm d}\langle\mathbf{x}^2\rangle}{{\rm d}t} &= -\frac{2\kappa\langle\mathbf{x}^2\rangle}{1+\lambda}+\frac{2\langle\mathbf{x}\cdot\mathbf{f}\rangle}{1+\lambda}+\frac{2d\lambda T}{(1+\lambda)^2},\\
\frac{{\rm d}\langle\mathbf{x}\cdot\mathbf{f}\rangle}{{\rm d}t} &= -\left[\frac{\kappa}{1+\lambda}+\frac{1}{\tau}\right]\langle\mathbf{x}\cdot\mathbf{f}\rangle+\frac{\langle\mathbf{f}^2\rangle}{1+\lambda},\\
\frac{{\rm d}\langle\mathbf{f}^2\rangle}{{\rm d}t} &= -\frac{2\langle\mathbf{f}^2\rangle}{\tau}+\frac{2dT}{\tau^2}.
\end{aligned} \tag{S15}$$

Owing to the linearity of (S15), the tracer variance during the compression interval $[0,\Delta t/2]$ can be deduced as follows. First, we integrate the self-propulsion variance as

$$\langle\mathbf{f}^2(t)\rangle = \langle\mathbf{f}^2(0)\rangle{\rm e}^{-t/2\tau}+\frac{dT}{\tau}\big(1-{\rm e}^{-t/2\tau}\big), \tag{S16}$$

which can be written as

$$\langle\mathbf{f}^2(t)\rangle = \langle\mathbf{f}^2(0)\rangle\mathbb{M}_{33}(t)+\mathbb{A}_3(t). \tag{S17}$$

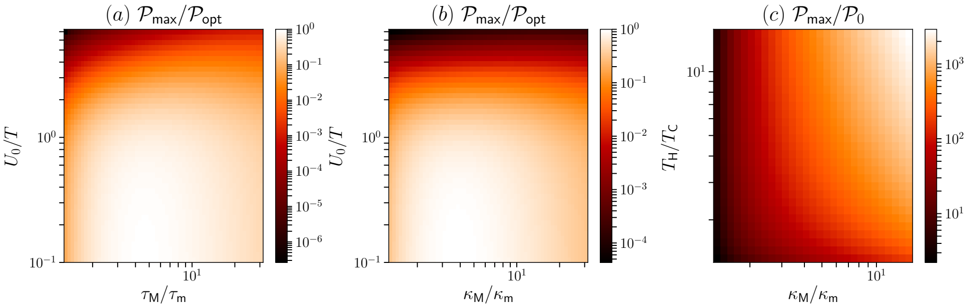


Fig. S1: Engine B: Maximum power $\mathcal{P}_{\max}$ scaled by the optimal value $\mathcal{P}_{\rm opt}$, (a) as a function of the scaled coupling with the bath $U_0/T$ and of the stiffness ratio $\kappa_{\rm M}/\kappa_{\rm m}$, and (b) as a function of the scaled coupling with the bath $U_0/T$ and of the persistence ratio $\tau_{\rm M}/\tau_{\rm m}$. Parameter values are the same as for Fig. 2(b) of the main text. Engine A: (c) $\mathcal{P}_{\max}$ as a function of the ratio between the maximum and the minimum values of stiffnesses $\kappa_{\rm M}/\kappa_{\rm m}$ and of temperatures $T_{\rm H}/T_{\rm C}$, in the absence of coupling with the bath. The scaling $\mathcal{P}_0$ corresponds to the case of a non-interacting passive tracer for the same values of $T_{\rm H}/T_{\rm C}$ and $\kappa_{\rm M}/\kappa_{\rm m}$ as in Fig. 1(b). Other parameter values are the same as for Fig. 1(b) of the main text.

The self-propulsion/tracer correlation and tracer variance then follow as

$$\begin{aligned} \langle \mathbf{x}\cdot\mathbf{f}(t)\rangle &= \langle \mathbf{x}\cdot\mathbf{f}(0)\rangle\mathbb{M}_{22}(t) + \langle \mathbf{f}^2(0)\rangle\mathbb{M}_{23}(t) + \mathbb{A}_2(t), \\ \langle \mathbf{x}^2(t)\rangle &= \langle \mathbf{x}^2(0)\rangle\mathbb{M}_{11}(t) + \langle \mathbf{x}\cdot\mathbf{f}(0)\rangle\mathbb{M}_{12}(t) + \langle \mathbf{f}^2(0)\rangle\mathbb{M}_{13}(t) + \mathbb{A}_1(t), \end{aligned} \tag{S18}$$

where $0 < \mathbb{M}_{ij}(t) < 1$. Likely, the correlations during the expansion interval $[\Delta t/2, \Delta t]$ can be cast in the form

$$\begin{aligned} \langle \mathbf{f}^2(t)\rangle &= \langle \mathbf{f}^2(\Delta t/2)\rangle\mathbb{N}_{33}(t) + \mathbb{B}_3(t), \\ \langle \mathbf{x}\cdot\mathbf{f}(t)\rangle &= \langle \mathbf{x}\cdot\mathbf{f}(\Delta t/2)\rangle\mathbb{N}_{22}(t) + \langle \mathbf{f}^2(\Delta t/2)\rangle\mathbb{N}_{23}(t) + \mathbb{B}_2(t), \\ \langle \mathbf{x}^2(t)\rangle &= \langle \mathbf{x}^2(\Delta t/2)\rangle\mathbb{N}_{11}(t) + \langle \mathbf{x}\cdot\mathbf{f}(\Delta t/2)\rangle\mathbb{N}_{12}(t) + \langle \mathbf{f}^2(\Delta t/2)\rangle\mathbb{N}_{13}(t) + \mathbb{B}_1(t), \end{aligned} \tag{S19}$$

with $0 < \mathbb{N}_{ij}(t) < 1$. Introducing the correlation vector $\mathbb{C}(t) = \big[\langle \mathbf{x}^2(t)\rangle, \langle \mathbf{x}\cdot\mathbf{f}(t)\rangle, \langle \mathbf{f}^2(t)\rangle\big]$, Eqs. (S17), (S18) and (S19) can be written as

$$\begin{aligned} t \in [0, \Delta t/2]: &\quad \mathbb{C}(t) = \mathbb{M}(t)\mathbb{C}(0) + \mathbb{A}(t), \\ t \in [\Delta t/2, \Delta t]: &\quad \mathbb{C}(t) = \mathbb{N}(t)\mathbb{C}(\Delta t/2) + \mathbb{B}(t). \end{aligned} \tag{S20}$$

The correlations in the expansion and compression branches are parametrized by the values at the beginning of each respective branch. In steady state, the values at the beginning of the compression and at the end of the expansion should be equal: $\mathbb{C}_{\rm S} = \mathbb{C}(0) = \mathbb{C}(\Delta t)$, which can be deduced explicitely from (S20) as

$$\mathbb{C}_{\rm S} = [\mathbb{I} - \mathbb{N}(\Delta t)\mathbb{M}(\Delta t/2)]^{-1}[\mathbb{N}(\Delta t)\mathbb{A}(\Delta t/2) + \mathbb{B}(\Delta t)], \tag{S21}$$

where $\mathbb{I}$ refers to the unit matrix. As a result, Eqs. (S20) and (S21) completely determine the time evolution of the tracer variance for a given value of the cycle time $\Delta t$, from which we deduce the extracted work $\mathcal{W}$ and the output power $\mathcal{P} = -\mathcal{W}/\Delta t$ as functions of $\Delta t$. In practice, we integrate numerically (S15) and let the system converge towards its steady state to determine $\mathbb{C}_{\rm S}$. Finally, we optimize the power as a function of cycle time to extract the maximum value $\mathcal{P}_{\max}$ for a given set of parameters, as reported in Fig. S1.

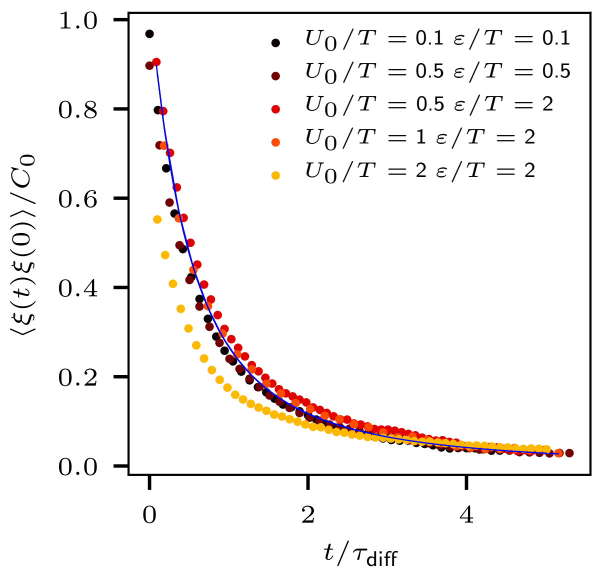


Fig. S2: Scaled correlations of the force exerted by the bath on the tracer projected $\langle\xi(t)\xi(0)\rangle/C_0$, where $C_0 = \pi\rho_0 U_0^2 T/2(T+\rho_0 V_{|\mathbf{k}=0})$, as a function of scaled time $t/\tau_{\text{diff}}$, where $\tau_{\text{diff}} = \sigma^2/\mu(T+\rho_0 V_{|\mathbf{k}|=0})$. The solid blue line refers to the analytic prediction (S11). Parameter values: $\rho_0 = \sigma = a = 1$, $\mu = 10$, $T = 1$, $\kappa = 0.5$.

**Numerical simulations.** – We consider interactions among bath particles through a pair-wise potential of the form $V(\mathbf{r}) = \varepsilon(1 - r/a)^2\Theta(a - r)$ in two dimensions, yielding $V_{|\mathbf{k}|=0} = \pi a^2\varepsilon/6$. We use Euler time-stepping to simulate the microscopic dynamics:

$$\begin{aligned}
\dot{\mathbf{x}} &= -\kappa\mathbf{x} - \nabla_{\mathbf{x}}\sum_i U(\mathbf{x}-\mathbf{r}_i) + \mathbf{f},\\
\dot{\mathbf{r}}_i &= -\mu\nabla_i\Big[\sum_j V(\mathbf{r}_i-\mathbf{r}_j) + U(\mathbf{x}-\mathbf{r}_i)\Big] + \boldsymbol{\eta}_i,\\
\tau\dot{\mathbf{f}} &= -\mathbf{f} + \boldsymbol{\zeta},
\end{aligned} \tag{S22}$$

where $\{\boldsymbol{\eta}_i\}$ and $\boldsymbol{\zeta}$ are uncorrelated zero-mean Gaussian noises with respective correlations $\langle\eta_{i\alpha}(t)\eta_{j\beta}(0)\rangle = 2\mu T\delta_{ij}\delta_{\alpha\beta}\delta(t)$, and $\langle\zeta_\alpha(t)\zeta_\beta(0)\rangle = 2T\delta_{\alpha\beta}\delta(t)$. The integration time is taken as equal to or smaller than $dt/\tau_{\text{diff}} = 10^{-3}$. We use periodic boundary conditions in a box of size $L = 25a$. The initial configuration is taken as homogeneous and random, measurements are taken after a waiting time of at least $t/\tau_{\text{diff}} = 10^2$. The harmonic trap applied on the tracer is centred at the middle of the box. To avoid boundary issues associated with confinement, we discard any realization where the tracer particle crosses the system boundaries.

To test the validity of the bath linearisation (S2), we compare measurements of the correlations of the force exerted by the bath on the tracer with our prediction (S11) for different strengths of the bath-bath and tracer bath-interactions, as reported in Fig. S2. Our results support that the linearisation is no longer valid for $U_0/T > 1$ and $\varepsilon/T > 1$, as expected. Parameter values used for the figures in the main text:

- Fig. 1(c): $\rho = \sigma = a = 1$, $\mu = 3$, $T_{\text{C}} = 1$, $T_{\text{H}} = 1.4$, $\kappa_{\text{m}} = 0.5$, $\kappa_{\text{M}} = 0.75$, $\varepsilon = 2$,
- Fig. 1(d): $\rho = \sigma = a = 1$, $\mu = 10$, $T_{\text{C}} = 1$, $T_{\text{H}} = 2$, $\kappa_{\text{m}} = 0.5$, $\kappa_{\text{M}} = 0.75$, $\varepsilon = 2$,

- Fig. 2(c): $\rho = \sigma = a = 1$, $\mu = 1$, $T = 1$, $\tau_{\rm m} = 1$, $\kappa_{\rm m} = 0.5$, $\kappa_{\rm M} = 0.75$, $U_0 = 1$, $\varepsilon = 2$,
- Fig. 2(d): $\rho = \sigma = a = 1$, $\mu = 1$, $T = 1$, $\tau_{\rm m} = 1$, $\tau_{\rm M} = 4.5$, $\kappa_{\rm m} = 0.5$, $U_0 = 1$, $\varepsilon = 2$.

REFERENCES

[1] Dean D. S., *J. Phys. A: Math. Gen.*, **29** (1996) L613.
[2] Démery V., Bénichou O. and Jacquin H., *New J. Phys.*, **16** (2014) 053032.
[3] Dean D. S. and Démery V., *J. Phys: Condens. Matter*, **23** (2011) 234114.
[4] Kubo R., *Rep. Prog. Phys.*, **29** (1966) 255.
